# Supplementary material for: LTLf Synthesis Under Environment Specifications for Reachability and Safety Properties
Source: arXiv:2308.15184 source file (2023-08-29)
Supplement: Supplementary file 1 [file 8-appendix.tex]

% This is samplepaper.tex, a sample chapter demonstrating the
% LLNCS macro package for Springer Computer Science proceedings;
% Version 2.21 of 2022/01/12
%

\appendix
\section{Appendix }

\subsection{Preliminaries}
\begin{remark} 
Linear temporal logic (\LTL)~\cite{Pnueli77} has the same syntax as \LTLf, and its semantics is over infinite traces. Thus, \LTL formulas denote properties. In particular, every reachability (resp. safety) property expressible in \LTL is expressible as $\exists \varphi$ (resp. $\forall \varphi$) for some \LTLf formula $\varphi$~\cite{DDTVZ21}.
\end{remark}

For example, let $\varphi_1,\varphi_2$ be \LTLf formulas. 

\begin{compactitem}
    \item 
    $\pi \models \exists \varphi_1 \land \forall \varphi_2$ iff some prefix of $\pi$ satisfies $\varphi_1$ and all prefixes of $\pi$ satisfy $\varphi_2$. 
    \item 
    $\pi \models \exists (\varphi_1 \land \varphi_2)$ iff some prefix of $\pi$ satisfies both $\varphi_1$ and $\varphi_2$.
\end{compactitem}

\setcounter{theorem}{1}

\subsection{Building Blocks for the Algorithms}

\paragraph{Preimage.} 
In order to compute the set of states from which the agent/environment can force a visit to a given set $S$ in one step, we need to define the \emph{controllabe/uncontrollable preimage}, which is the main step for solving reachability and safety games.
We define the controllable preimage $Pre_\ag(E)$ of a set $E\subseteq Q$ as the set of states, from which there exists an agent action $Y \in 2^\Y$ such that for all environment response $X \in 2^\X$, the corresponding successor state $\delta(q,X \cup Y)$ is in $E$. Analogously, $Pre_\env(E)$ denotes the set of states, from which for all $Y \in 2^\Y$, there exists $X \in 2^\X$ such that $\delta(q,X \cup Y)$ is in $E$. Formally,
\begin{align*}
    Pre_\ag(E)= & \{q \in Q| \exists Y \forall X.\delta(q,X \cup Y) \in E\} \\
    Pre_\env(E)= & \{q \in Q| \forall Y \exists X.\delta(q,X \cup Y) \in E\}
\end{align*}

\paragraph{Reachability Games.} Given a game arena $\D= (\Sigma, Q, \iota,\delta)$ and a reachability condition $(\reach,T)$,   \textsc{Solve$_\ag(\D,\reach,T)$}  solves the reachability game over $\D$ for the agent  by computing  the least fixed-point as follows. 
\begin{align*}
&\Z_0(\D) = T \label{eq:win0} \\ 
&\Z_{i+1}(\D) = \Z_i(\D) \cup Pre_\ag(\Z_i(\D))
\end{align*}

The computation reaches a fixed point when $\Z_i = \Z_{i+1}$, hence $\Z = \Z_{i+1}$ collects all the winning states for the protagonist. If $\iota \in \Z$, we compute a positional strategy as follows. Define $f_\ag: Q \rightarrow 2^\Y$  such that
for every $q \in \Z \setminus \Z_0$, if $q$ is added for the first time in the $(i+1)$-$th$ iteration of the fixpoint computation (i.e.,  $q \in \Z_{i+1} \backslash \Z_{i}$),  define $f_\ag(q) = Y$, where $Y$ is any element such that $\forall X \in 2^\X. \delta(q, Y\cup X)\in \Z_{i}$ (If there is more than one such $Y$, arbitrarily choose one); if $q  \in \Z_0$ or $q\not \in \Z$, define $f_\ag(q)$ arbitrarily. % for some (arbitrary) $Y \in 2^{\Y}$.

\sr{new}
\begin{lemma} \label{lem:solvereach}
The procedure $\textsc{Solve}_\ag(\D,\reach(T))$ returns the winning region $W_\ag$ and a function $w_\ag$ such that the agent strategy $\textsc{Strategy}(w_\ag)$ wins the game $(\D,\reach(T))$.
\end{lemma}

Solving the reachability game considering the environment as the protagonist can be defined analogously, in particular replacing $Pre_\ag(\Z_i(\D))$ by $Pre_\env(\Z_i(\D))$. In this case, the positional strategy $f_\env: Q \times 2^Y \rightarrow 2^\X$ is such that for every $q \in \Z_{i+1} \backslash \Z_{i}$ and $Y \in 2^\Y$, $f_\env(q, Y) = X$, where $X$ holds that $\delta(q, Y\cup X)\in \Z_{i}$ (Similarly, if there is more than one such $X$, arbitrarily choose one). Moreover, if $q \in \Z_0$ or $q \not \in \Z$,  $f_\env(q,Y)=X$, for  $Y \in 2^\Y$ and $X \in 2^\X$.

\paragraph{Safety Games.} Given a game arena $\D= (\Sigma, Q, \iota,\delta)$ and a safety condition $(\safe,T)$, \textsc{Solve$_\ag(\D,\safe, T)$}  solves the safety game over $\D$, considering the agent as the protagonist, by computing the greatest fixed point as follows: 
\begin{align*}
&\Z_0(\D) = T  \\
&\Z_{i+1}(\D) = \Z_i(\D) \cap Pre_\ag(\Z_i(\D))
\end{align*}

Solving the safety game considering the environment as the protagonist $\textsc{Solve}_\env$ can be defined analogously by replacing $Pre_\ag(\Z_i(\A))$ with $Pre_\env(\Z_i(\A))$.

The computation reaches fixpoint when $\Z_i = \Z_{i+1}$, hence $\Z = \Z_{i+1}$ collects all the winning states for the protagonist. If $\iota \in \Z$, we compute a positional strategy as follows. Considering the agent as the protagonist, we have $f_\ag: Q \rightarrow 2^\Y$ such that for every $q \in \Z$, $f_\ag(q) = Y$, where $Y$ holds that $\forall X \in 2^\X. \delta(q, Y\cup X)\in \Z$ (If there are more than one such $Y$, arbitrarily choose one). For the case of the environment being the protagonist, the positional strategy $f_\env: Q \times 2^Y \rightarrow 2^\X$ is such that for every $q \in \Z$ and $Y \in 2^\Y$, $f_\env(q, Y) = X$, where $X$ holds that $\delta(q, Y\cup X)\in \Z$ (If there are more than one such $X$, arbitrarily choose one). 
\begin{comment}
We summarise this as follows:
\begin{lemma} \label{lem:solvesafe}
The procedure $\textsc{Solve}_\ag(\D,\safe,T)$ returns the winning region $W$ and a winning strategy $f_\ag$ that wins from every winning state.
\end{lemma}
\end{comment}
\begin{remark}\label{rm:allsafestrategies} 
Given a transition system $\D$ with state set $Q$, and a set $T \subseteq Q$, consider the safety \DA $\A = (\D,\safe(T))$. Let $\Win_p$ be the winning region of the protagonist. Consider the restricted transition system $\D' := \textsc{Restrict}(\D, \Win_p)$. Note that $\A' = (\D',\safe(T))$ is a well-defined \DA (i.e., reaching the $sink$ violates the safety condition). A strategy for the protagonist is winning in $\A$ iff it is winning in $\A'$. Intuitively, this is because winning strategies for a safety condition cannot leave the winning region, and this is the only requirement for them to be winning. Thus, intuitively, the restriction $\D'$ represents all the strategies that enforce $\L(\D,\safe,T)$~\cite{BernetJW02}.
\end{remark}
%\appendix
\section{Appendix : Proofs}

\begin{theorem}
   Let each of \Task and \Env be of the forms $\forall \varphi$, $\exists \varphi$, or $\exists \varphi_1 \land \forall \varphi_2$. Solving synthesis for an agent \Task under  environment specification \Env
 is 2EXPTIME-complete. 
\end{theorem}

\begin{proof}
    \emph{Upper Bound.} The solutions provided in Algorithms 1-7 rely on constructing the corresponding \DFAs of \Task and \Env, cartesian products of a bounded number of \DFAs, as well as solving reachability and safety games.
    The corresponding \DFAs of \Task and \Env can be constructed in 2EXPTIME in the size of \Task and \Env, and solving reachability and safety games can be accomplished in polynomial time in the size of the \DFA. 
    %Moreover, cartesian products of \DFAs are polynomial in the size of the \DFAs.
    In summary, the upper bound for Algorithms 1-7 is 2EXPTIME.
    
    \emph{Lower Bound.} The following problem is known (see~\cite{DegVa15}) to be 2EXPTIME-hard (*): given an \LTLf formula $\varphi$ decide if there exists an agent strategy that enforces $\exists \varphi$. Thus, e.g., we get hardness for synthesis for $\Task = \exists \varphi_1 \land \forall \varphi_2$ under $\Env = \true$ (just let $\varphi_2 = \true)$. To handle the missing cases, we will show that the following problem is 2EXPTIME-hard (+): given an \LTLf formula $\varphi$ decide if there is an agent strategy that enforces $\forall \varphi$. 
    
    First note that if $L$ is in 2EXPTIME, then so is $L^c$, the complement of $L$ (this is because 2EXPTIME is a deterministic complexity class). Thus, if $L$ is 2EXPTIME-hard, then so is $L^c$ (indeed, if $X$ is in 2EXPTIME, then so is $X^c$, which reduces to $L$ by assumption, and thus $X$ reduces to $L^c$). Thus, by (*), we have that the following problem is 2EXPTIME-hard: given an \LTLf formula $\varphi$ decide if there does \emph{not} exist an agent strategy that enforces $\exists \varphi$. By determinacy of the corresponding game~\cite{Mar75}, there does not exist an agent strategy that enforces $\exists \varphi$ if and only if there exists an environment strategy that enforces $\forall \lnot \varphi$. Thus, we have that the following problem is 2EXPTIME-hard (**): given an \LTLf formula $\varphi$, decide if there is an environment strategy that enforces $\forall \varphi$. To finish the proof, we reduce (**) to (+). Take an instance $\varphi$ of $(**)$; suppose $AP = X \cup Y$ where the agent controls the variables in $Y$ and the environment controls the variables in $X$. Define $AP' = X \cup Y \cup Y'$ where $Y' = \{y': y \in Y\}$ (i.e., $Y'$ is a copy of $Y$, call its elements 'primed'), and let the agent control the variables in $X$ and the environment control the variables in $Y$. Define
    \[
    \varphi' = (\Wnext \false) \lor (( \Box \wedge_{y \in Y} (y' \limp \Wnext y)) \limp (\Next \varphi))
    \]
  %  The meaning of $\varphi'$ is as follows: either the trace has length equal to $1$, or if the environment correctly copies its moves to the successors (and unprimes them) the formula $\varphi$ holds from the second time-step onwards. 
  It is not hard to see that the environment can enforce $\forall \varphi$ iff the agent can enforce $\forall \varphi'$. Intuitively, this is because the new objective $\varphi'$ checks if $\varphi$ holds from the second step onwards as long as the environment correctly copies and unprimes its moves from each previous time-step.
\end{proof}

\begin{theorem}%\label{thm:alg-safety}
Algorithm~\ref{alg:reach} solves the synthesis under environment specifications problem with $\Task = \exists \varphi,\Env = \true$.
\end{theorem}

\sr{i added a new proof.}
\begin{proof}
By Lemma 1, we have (*): $L(\D,\reach(T))=L(\exists \varphi)$. 

Suppose $\iota \in W$. We must show that the agent strategy $\sigma_\ag = \textsc{Strategy}(f_\ag)$ returned by the algorithm enforces $\exists \varphi$. So, let $\pi$ be a trace that follows $\sigma_\ag$ (we will show that $\pi \models \exists \varphi$). By Lemma~\ref{lem:solvereach}, $\sigma_\ag$ wins the game $(\D,\reach(T))$. By Definition~\ref{dfn:agent strategy wins game}, this means that $\pi \in L(\D,\reach(T))$. By (*), $\pi \in L(\exists \varphi)$.

Conversely, suppose $\iota \not \in W$. The algorithm returns "unrealisable", and we must show that there is no agent strategy that enforces $\exists \varphi$. Suppose towards a contradiction that there were, call it $\sigma$. By determinacy (Lemma~\ref{lemma:determined}), there is an environment strategy $\sigma_\env$ that wins the game $(\D,\reach(T))$ for the antagonist. By definition this means that for every trace $\pi$ that follows $\sigma_\env$, the run of $\pi$ on $\D$ satisfies that $\pi_i \not \in T$ for every $i$, and thus $\pi \not \in L(\D,\reach(T))$, and so by (*) $\pi \not \models \exists \varphi$. But if $\sigma$ enforces $\exists \varphi$ then $\pi=\play(\sigma,\sigma_\env) \models \exists \varphi$, a contradiction. \sr{an alternative approach for this second part is to show that the environment has a strategy that enforces $\lnot \exists \varphi$. This should follow from a dual to Lemma 2...}
\end{proof}

\begin{proof}[Old]
By Lemma~\ref{lem:autconstruction}, the language of the \DA in Line 1 is $\L(\exists \varphi)$. 
By Lemma~\ref{lem:games-synthesis} it is enough to find check $\iota$ is a winning state, and in this case to compute a winning strategy $f_\ag$ and return $\textsc{Strategy}(f_\ag)$. But finding the winning region and a winning strategy (for every state in the winning region) for reachability games is done in Line 2.% \cite{}.
%using Lemma~\ref{lem:solvereach}.
\end{proof}

\begin{theorem}%\label{thm:alg-safety}
Algorithm~\ref{alg:safe} solves the synthesis under environment specifications problem with $\Task = \forall \varphi,\Env = \true$.
\end{theorem}

\begin{proof}
By Lemma \ref{lem:autconstruction}, the language of the \DA in Line 1 is $\L(\forall \varphi)$.
By Lemma~\ref{lem:games-synthesis} it is enough to find check $\iota$ is a winning state, and in this case to compute a winning strategy $f_\ag$ and return $\textsc{Strategy}(f_\ag)$. But finding the winning region and a winning strategy (for every state in the winning region) for safety games is done in Line 2.
%in Line 2 using Lemma~\ref{lem:solvereach}.
\end{proof}

\begin{theorem}%\label{thm:reachsafe}
Algorithm~\ref{alg:reachsafe} solves synthesis under environment specifications problem with $\Task = \exists \varphi_1 \land \forall \varphi_2,\Env = \true$.
\end{theorem}

\begin{proof}
%By Lemma \ref{lem:autconstruction}, the language of the \DA in Line 1 is $\L(\exists \varphi_1)$, and the language of the \DA in Line 2 is $\L(\forall \varphi_2)$.
%Let  $S_1$  be the agent winning region in the safety game over $\D_{\forall \varphi_2}$, we have that $S_1$ represents  the set of winning strategies for the agent enforcing $\forall \varphi_2$.
%Restricting all the environment strategies to consider only those
%that enforce $L(\forall \varphi_2)$ is done in Line 5 using Lemma \ref{lem:lift strategies to product}. By Lemma 2 it is enough to check $\iota$ is a winning state, and in this case to compute a winning strategy $f_\ag$ and return  $\textsc{Strategy}(f_\ag)$.

---
%By Lemma \ref{lem:autconstruction}, the language of the \DA in Line 1 is $\L(\exists \varphi_1)$, and the language of the \DA in Line 2 is $\L(\forall \varphi_2)$. 

We want to show that if $\sigma_\ag$ is winning in $(\D_{\exists \varphi_1} \times \D_{\forall \varphi_2}, \reach, T_1 \times S_2)$ then $\sigma_\ag \rhd  \varphi_1 \land \forall \varphi_2$. 
First, we have that, by Lemma \ref{lem:autconstruction}, $\pi \models \exists \varphi_1$ iff $\pi \in \L(\D_{\exists \varphi_1}, \reach,T_1)$ iff, by Lemma 4, $\pi \in \L(\D_{\exists \varphi_1} \times \D_{\forall \varphi_2}' , \reach,T_1 \times S_2)$. Note that, by construction, $\pi$ follows $g_\ag$ until a state $q \in T_1 \times S_2$ is reached. Moreover, no $sink$ state is visited.
We need to show that $\pi \models \forall \varphi_2$. Since $\sigma_\ag$ is winning in $(\D_{\exists \varphi_1} \times \D_{\forall \varphi_2}, \reach, T_1 \times S_2)$, we have that, after reaching $q \in T_1 \times S_2$, $\pi$ follows $f_\ag''$ and the projection of $q$ on the components from $Q_2$ is in $S_2$. Therefore,  $\pi \in \L(\D_{\exists \varphi_1} \times \D_{\forall \varphi_2},\safe, T_1 \times S_2$. We know that  $\pi \models \forall \varphi_2$  by Lemma \ref{lem:autconstruction}, $\pi \models \forall \varphi_2$ iff $ \pi \in \L(\D_{\forall \varphi_2},\safe, T_2)$ iff, by Lemma 5,  $ \pi \in \L(\D_{\forall \varphi_2}',\safe, S_2)$ iff, by Lemma 4,  $ \pi \in \L(\D_{\exists \varphi_1} \times \D_{\forall \varphi_2}',\safe, T_1 \times S_2)$. This concludes the proof.
%from $q \in \iota$ until a state $q \in T_1 \times S_2$ is reached. 
%We need to show that $\pi \models \exists \varphi_1$. 

%
%We need to show that $\pi \models \forall \varphi_2$. 

%\in \R$, the projection of $q$ on the components from $Q_2$ is in $S$, hence $\pi \in \L(\A_2)$. 
%In particular, we need to show that any state in $\pi$ does not visit a sink state. 
%
%Let $\pi$ be a trace that starts at $\iota$ and follows $g_\ag$. Since $q^\C_0 \in \R$, $\pi \in \L(\A_3)$ holds. 

\end{proof}

\begin{lemma}[\cite{}]\label{restriction}
Let $\A=(\D,safe,T)$ be a \DA and $S$ the set of winning states for the protagonist in the safety game over $\A$. Let $\A'=(\D',safe,S)$ be the restriction of $\A$. Then every winning strategy for the protagonist in the safety game over $\A$ is a winning strategy in the safety game over $\A'$, and viceversa.
\end{lemma}

%\begin{theorem}[\cite{BJW02}]
%Let $\A$ be a safety game. We have that if the protagonist $p$ has a winning strategy in $\A$, then $p$ has a maximal permissive strategy that is \emph{memoryless}, i.e., $\sigma_p: Q \rightarrow 2^{2^\Y}$.
%\end{theorem}

\begin{theorem}%\label{thm:alg-correct}
Algorithm~\ref{alg:safe->reach} solves the synthesis under environment specifications problem with $\Task = \exists \varphi_1, \Env = \forall \varphi_2$.
\end{theorem}
\begin{proof}

We show that  $\sigma_\ag$ returned by Algorithm \ref{alg:safe->reach} is winning in $(\D, \reach,(T_1 \times S_2) \cup (Q_1 \times \{\bot\})$ iff   $\sigma_\ag \ \rhd_\Env \Task$.

%$\rightarrow$. 
We need to show that for every $\sigma_\env \rhd \Env$, $\pi =\play(\sigma_\ag,\sigma_\env) \models \Task$.
By Lemma~\ref{lem:autconstruction}, the language of the \DA $\A_1 = (\D_1, \reach,T_1)$ in Line 1 is $\L(\exists \varphi_1)$ and the language of the \DA $\A_2 = (\D_2, \safe,T_2)$ in Line 2 is $\L(\forall \varphi_2)$. 

Take an environment strategy $\sigma_\env \rhd \Env$. We have that, by Lemma 1,  $\pi \models \Env$ iff $\pi \in \L(\D_2,safe, T_2)$, by Lemma 5,  iff $ \pi \in \L(\D_2',safe,S_2)$, by Lemma 4, iff $\pi \in \L(\D_1\times \D_2',safe,T_1 \times S_2)$.

Now, we need to show that $\pi \models \Task$.  $\sigma_\ag$ is winning in $(\D, \reach, (T_1 \times S_2) \cup (Q_1 \times \{\bot\})$ then, by Lemma 2, $\pi \in \L(\D, \reach, (T_1 \times S_2) \cup (Q_1 \times \{\bot\}))$. However, $\pi \models \Env$, then we need to show that $\pi \in \L(\D, \reach, T_1 \times S_2)$ and $\pi \not\in \L(\D, \reach,Q_1 \times \{\bot\})$. We have that, $\pi \models \Task$ iff $\pi \in \L(\D_1,\reach,T_1)$, by Lemma 1, iff $\pi \in \L(\D_1 \times \D_2',\reach,T_1 \times S_2)$, by Lemma 4.
Then, $\pi \models \Task$. 
Moreover, we have that if $\pi \in \L(\D_2', \safe, S_2)$ then $\pi \not \in \L( \D_2', \reach, \{\bot\})$, and by Lemma 4, $\pi \not \in \L(\D_1 \times D_2', \reach, Q_1 \times \{\bot\})$. This concludes the proof.
\end{proof}

\begin{theorem}%\label{thm:alg-correct}
Algorithm~\ref{alg:safe->safe} solves the synthesis under environment specifications problem with $\Task = \forall \varphi_1, \Env = \forall \varphi_2$.
\end{theorem}
\begin{proof}
By Lemma~\ref{lem:autconstruction}, the language of the \DA $A_1 = (\D_1, \safe, T_1)$ in Line 1 is $\L(\forall \varphi_1)$ and the language of the \DA $A_2 = (\D_2, \safe, T_2)$ in Line 2 is $\L(\forall \varphi_2)$. Finding all the environment strategies that enforce $\L(\A_2)$ through safety games considering the environment as the protagonist is done in Lines 3\&4 
%using Lemma~\ref{lem:solvesafe} 
Remark~\ref{rm:allsafestrategies}. Restricting all the environment strategies to considering only those that enforce $\L(\A_2)$ is done in Line 5 using Lemma~\ref{lem:lift strategies to product}. By Lemma~\ref{lem:games-synthesis} it is enough to find check $\iota$ is a winning state, and in this case to compute a winning strategy $f_\ag$ and return $\textsc{Strategy}(f_\ag)$. But finding the winning region and a winning strategy (for every state in the winning region) for safety games is done in Line 6.% using Lemma~\ref{lem:solvesafe}.
\end{proof}

\begin{theorem}%\label{thm:alg-correct}
Algorithm~\ref{alg:safe->reach+safe} solves synthesis under environment specifications problem with $\Task = \exists \varphi_1 \land \forall \varphi_2, \Env = \forall \varphi_3$.
\end{theorem}
\begin{proof}
By Lemma~\ref{lem:autconstruction}, the language of the \DA $A_1 = (\D_1, \reach,T_1))$ in Line 1 is $\L(\exists \varphi_1)$, the language of the \DA $A_2 = (\D_2, \safe, T_2)$ in Line 2 is $\L(\forall \varphi_2)$, and the language of the \DA $A_3 = (\D_3, \safe,T_3)$ in Line 1 is $\L(\forall \varphi_3)$. Finding all the environment strategies that enforce $\L(\A_3)$ through safety games considering the environment as the protagonist is done in Lines 4\&5 using %Lemma~\ref{lem:solvesafe} and 
Remark~\ref{rm:allsafestrategies}. Restricting all the environment strategies to considering only those that enforce $\L(\A_3)$ is done in Line 6 using Lemma~\ref{lem:lift strategies to product}. Finding all the agent strategies that realize $\A_2$ under environment specification $\A_3$ through safety games is done in Lines 7\&8 using %Lemma~\ref{lem:solvesafe} and 
Remark~\ref{rm:allsafestrategies}. Note that this step also returns one agent strategy $f^s_\ag$.
Restricting all the environment strategies to considering only those that enforce $\L(\A_3)$ and agent strategies to considering only those that realize $\A_2$ under environment specification $\A_3$ is done in Line 9 using Lemma~\ref{lem:lift strategies to product}. Finding the winning region and a winning strategy $f^r_\ag$ (for every state in the winning region) for reachability games is done in Line 10.
%using Lemma~\ref{lem:solvereach}. 
By Lemma~\ref{lem:games-synthesis} it is enough to check $q^\C_0$ is a winning state, and in this case to compute a winning strategy $f_\ag$ by combining strategies $f^s_\ag$ and $f^r_\ag$
and return $\textsc{Strategy}(f_\ag)$. The correctness of $\textsc{Combine}(\C, S, f^s_\ag, R, f^r_\ag)$ is shown by construction: let $\pi$ be a trace that starts at $q^\C_0$ and follows $f_\ag$. Since $q^\C_0 \in \R$, $\pi \in \L(\A_3)$ holds. Moreover, note that for $q \in \R$, the projection of $q$ on the components from $Q_2$ is in $S$, hence $\pi \in \L(\A_2)$. 
\end{proof}

\setcounter{lemma}{6}

\begin{lemma}\label{lem:alg7}
To solve any game with objective $(\eventually T) \lor \beta$ (for $\beta \subseteq Q^\omega$) proceed as follows:
\begin{compactenum}
\item Let $(M,m_\ag) = \textsc{Solve}(\D, \reach(T))$.
\item Let $\D'$ be the restriction of $\D$ to $Q \setminus M$ (this introduces a new $sink$ state).
\item Let $(N,n_\ag) = \textsc{Solve}(\D',\beta)$. 
\item Let $W = M \cup N$.
\item Define $f_\ag$ as follows: if the history ever enters $M$ follow $m_\ag$; if the starting state is in $N$, follow $n_\ag$; otherwise make an arbitrary move.
\end{compactenum}
\end{lemma}

\begin{proof}
To see that this is correct, let $\rho$ be a path in $\D$ that starts in $q \in W$ and is consistent with $f_\ag$. Note that if $\rho_i \in M$ for some $i$, then $\rho_{\geq i}$ is consistent with $m_\ag$ and thus is in $(\reach, T)$, and thus $\rho \in \reach(T)$. In particular, if $q \in M$ then $\rho \in \reach(T)$. If $q \in N$ then $\rho_i \in Q \setminus M$ for all $i$, and so it is consistent with $n_\ag$, and so satisfies $\beta$. Thus we have shown that $f_\ag$ enforces the objective from $W$. 

We must now show that the opponent enforces the negation of the objective, i.e., $(\always \lnot T) \land \lnot \beta$, from $Q \setminus W$. For this, let $f_\env$ be the opponent's strategy that enforces $\lnot \varphi$ in $\D'$, i.e., every play in $\D'$ consistent with $f_\env$ that starts in $Q \setminus W$ satisfies $\lnot \varphi$. Let $\rho$ be a path in $\D$ that starts in $q \in Q \setminus W$ and is consistent with $f_\env$. Note that the play stays in $\D'$ since $Q \setminus M$ is a trap for the player; thus $\rho$ satisfies $\always \lnot T$ (since $T \subseteq M$) and $\lnot \varphi$, as required. 
\end{proof}

\begin{theorem}%~\label{thm:reach+safe->reach+safe}
Algorithm~\ref{alg:reach+safe->reach+safe} solves the synthesis under environment specifications problem with $\Task = \exists\varphi_3 \land \forall \varphi_4$ and $\Env = \forall \varphi_1 \land \exists \varphi_2$.
\end{theorem}
\begin{proof}
By Lemma~\ref{lem:alg7}, it is enough to show that the algorithm correctly solves the game produced at the end of Line 8: the transition system is $\D'_p$ and the winning condition is $\safe(T_2) \cup (\safe(T_4) \cap \reach(T_3))$. First, note that Line 9 only refines the state space (by adding the flag component), and so it is enough to show that the rest of the algorithm correctly solves the game on $\D^f$ produced at Line 9.

To do this we will show that $f_\ag$ enforces $\alpha = \safe(T_2) \cup (\safe(T_4) \cap \reach(T_3))$ from $W_\ag$, and that the environment has a strategy $f_\env$ that enforces the complement of $\alpha$, i.e., $\overline{\safe(T_2)} \cap (\overline{\safe( T_4)} \cup \overline{\reach(T_3)})$, from the rest of the states.

Let $\rho$ be a path in $\D^f$ consistent with $f_\ag$. 
\begin{compactenum}
    \item 
    If $\rho$ starts in $S_2$ then it satisfies $\safe(T_2)$ since it uses $f^2_\ag$. 
    \item 
    If $\rho$ starts in $R_3$ then it satisfies $\reach(R_3) \cap \safe(T_4)$ since it uses $f^3_\ag$ followed by $f^4_\ag$. 
    \item 
    Suppose $\rho$ starts in $E$. If it stays in $V_0$ then it satisfies $\safe(T_2) \cap \safe(T_4)$, and thus $\safe(T_2)$, since it follows $f^e_\ag$. If it leaves $V_0$ then the corresponding path in $\D^f$ reaches $\top$. Let $s \in Q^f \setminus V_0$ be the target of this last transition in $\D^f$. Note that every state on the path up to (but not necessarily including $s$) is in $T_2 \cap T_4$. There are three cases. 
\begin{compactenum}
    \item 
    If $s \in S_2$ proceed as before and use $f^2_\ag$; since $T_2$ held up till now, $\rho \in \safe(T_2)$. 
    \item 
    If $s \in R_3$ proceed as before and use $f^3_\ag$ until $T_3$ is visited and then switch to $f^4_\ag$; since $T_4$ held up till now, $\rho \in \safe(T_4) \cap \reach(T_3)$. 
    \item 
    If $s \in (S_4 \setminus T_2) \setminus (R_3 \cup S_2)$ then the value of the flag at $s$ is $yes$ and thus $T_3$ was seen, so switch to $f^4_\ag$ to also ensure $\safe(T_4)$. 
\end{compactenum}
\end{compactenum}

To define the environment strategy $f_\env$ we need some strategies from the construction. 

\begin{compactitem}
    \item 
    Let $S'_2$ and ${f}^2_\env$ be the winning region and winning strategy in $\D^f$, respectively, for the environment in Line 10. So, a play that follows $f^2_\env$ from $S'_2$  violates $\safe(T_2)$.

    \item 
    Let $S'_4$ and $f^4_\env$ be the winning region and winning strategy in $\D^f$, respectively, for the environment in Line 11. 
    So, a play that follows $f^4_\env$ from $S'_4$ violates $\safe(T_4)$.  
    
    \item Let $R'_3$ and $f^3_\env$ be the winning region and winning strategy in $\D^f$, respectively, for the environment in Line 12. \sr{pedantics: we should lift this set and str to $\D^f$}
    So, a play that follows $f^3_\env$ from $R'_3$ will never visit $T_3$ if it stays in the restricted arena (Line 12), and if it leaves $S_4$ then it is in $S'_4$, a previous case in which the environment can violate $\safe(T_4)$.
    
    \item 
    Let $E'$ be such that $E' \cup \{\bot\}$ is the winning region for the environment in Line 16, and let $f^e_\env$ be a winning strategy. So, for a play that follows $f^e_\env$ starting in $E'$, if it stays in this domain then eventually a state is reached that is either not in $T_2$ or not in $T_4$, and if it leaves this domain it enters a state in $S_4 \setminus (R_3 \cup S_2 \cup T_2) = S_4 \setminus (R_3 \cup T_2)$ in which the value of the flag is $no$ meaning that $T_3$ has not been visited yet.
\end{compactitem}

Define $W_\env := Q^f \setminus W_\ag = (S_4 \setminus (R_3 \cup S_2 \cup T_2)) \cup E' = (S_4 \setminus (R_3 \cup T_2)) \cup E'$.
We now define $f_\env$. Suppose $q$ is the first state of the history. 
\begin{compactenum}
    \item 
    If $q \not \in W_\env$ then define $f_\env$ arbitrarily. 
    \item 
    If $q \in S_4 \setminus (R_3 \cup T_2)$ then in particular $q \not \in T_2$ and already $\safe(T_2)$ is violated so $f_\env$ follows $f^3_\env$ to ensure that $\reach(R_3)$ is violated (or if play leaves $S_4$ then $\safe(T_4)$ is violated). 
    \item If $q$ is in $E'$ then $f_\env$ follows $f^e_\env$. This ensures that eventually a state $s$ is reached such that at least one of the following cases hold:
    \begin{compactenum}
    \item 
    $s \not \in T_4$ (so in particular $\safe(T_4)$ is violated). Since $S_2$ is disjoint from $V$, let $f_\env$ switch to $f^2_\env$ so that $\safe(T_2)$ is violated.
    \item 
    $s \not \in T_2$ (so in particular $\safe(T_2)$ is violated). Since $S_4 \setminus T_2$ is disjoint from $V_0$, let $f_\env$ switch to $f^4_\env$ so that $\safe(T_4)$ is violated.
    \item $s \in S_4 \setminus (R_3 \cup T_2)$ and its flag value is $no$. In this case $f_\env$ switches to $f^e_\env$ and wins as if it started in this state (as above).
\end{compactenum}
\end{compactenum}
\end{proof}
